# Supplementary material for: Advancing Volumetric Medical Image Segmentation via Global-Local Masked Autoencoder
Source: arXiv:2306.08913 source file (2023-08-23)
Supplement: Supplementary file 1 [file Supp_experiments.tex]

\section{Experiments}\label{sec:exp}

\subsection{Implementation details}
\noindent\textbf{Datasets.}\label{sec:dataset}
We provide a detailed overview of the datasets that we utilized in our experiments. Consistent with prior research~\cite{chen2023masked,tang2022self}, as outlined in Table~\ref{tab:dataset}, the \textit{BTCV} and \textit{TCIA Covid} datasets were merged to create a pretraining unlabelled dataset $\mathcal{D}$, comprising 746 CT datasets focused on thoracic organs. Prior to being fed to the model, the data was normalized within the range of [0, 1], following a hue value of [-1000, 1000]. For our downstream tasks, we employed five distinct datasets that covered tasks such as multiple organ segmentation, whole heart segmentation, and COVID-19 lesion segmentation. While all other datasets were CT-based, \textit{BraTS} was an MRI dataset for further evaluating the generalization capability of our method. Following~\cite{tang2022self,chen2023masked}, we partitioned the datasets into training and validation subsets, based on the official split provided. However, given that the relevant organs differed across each downstream task, we employed different normalized value ranges.
\begin{table*}[thb]
	\centering
	\caption{The datasets used for pre-training and downstream fine-tuning include volumetric data of multiple organs.}
	\label{tab:dataset}
    \resizebox{0.88\linewidth}{!}{
	\begin{tabular}{ccccccc}
        \whline
		Datasets & Organ details & Modality & Train & Validation & Normalized Value \\
		\hline
		\textbf{\textit{Pre-training}} & & & & &\\
		BTCV~\cite{landman2015miccai} & Multiple chest organs & CT & 24 & - & [-1000, 1000]\\
		TCIA Covid19~\cite{an2020ct} & Multiple chest organs & CT & 722 & - & [-1000, 1000]\\
		\cdashline{1-6}
		\textbf{\textit{Fine-tuning}}  & & & & &\\
		BTCV~\cite{landman2015miccai} & Multiple chest organs & CT & 24 & 6 & [-175, 250] \\
		MSD Task 07~\cite{simpson2019large} &  Spleen & CT & 41 & 20 & [-57, 164]\\
		MM-WHS~\cite{zhuang2018multivariate} & Whole heart & CT & 16 & 4 & [0, 1700]\\
		BraTS~\cite{simpson2019large} & Brain tumor & MRI & 484 & 266& -\\ 
		Covid-19-20~\cite{roth2022rapid} & Chest diseases & CT& 160 & 39 & [-1000, 500]\\
        \whline
	\end{tabular}
 }
    % \\ \textsuperscript{*}{\raggedleft{Note: Spl: spleen, RKid: right kidney, LKid: left kidney, Gall: gallbladder, Eso: esophagus, Liv: liver, Sto: stomach, Aor: aorta, IVC: inferior vena cava, Veins: portal and splenic veins, Pan: pancreas, AG: left and right adrenal glands.}.}
    % MM-WHS contains 7 classes, including myocardium of LV (Myo), left ventricle (LV), left atrium (LA), right atrium (RA), right ventricle (RV), whole aorta (aorta) and pulmonary artery (PA)}
 
\end{table*}
 
\begin{table*}[htb]
    \centering
    \caption{The training details for the model on each dataset mostly followed the settings in the previous works.}
    \label{tab:configs}
    \resizebox{0.75\linewidth}{!}{
    \begin{tabular}{c|cccccc}
        \whline
         Config & Stetting & Learning Rate & Batch Size & Epochs & Cropped Size\\
         \midrule
         BTCV & Linear & 3e-4 & 4 & 3000 & $[96, 96, 96]$ \\
         BTCV & End-to-end & 3e-4 & 4 & 3000 & $[96, 96, 96]$ \\
         BTCV & Semi-Supervised & 1e-4 & 4 & 3000 & $[96, 96, 96]$ \\
         MM-WHS & End-to-end & 1e-3 & 2 & 600 & $[96, 96, 96]$ \\
         BraTS & End-to-end & 1e-4 & 1 & 300 & $[224, 224, 144]$\\
         Covid-19-20 & End-to-end & 1e-4 & 4 & 500 & $[192, 192, 16]$ \\
         MSD Task 07 & End-to-end & 1e-4 & 2 & 600 & $[96, 96, 96]$ \\
        \whline
    \end{tabular}}\\
    % \textsuperscript{*}{\raggedleft{MM-WHS contains 7 classes including myocardium of LV (Myo), left ventricle (LV), left atrium (LA), right atrium (RA), right ventricle (RV), whole aorta (aorta) and pulmonary artery (PA)}}
\end{table*}

\noindent\textbf{Finetuning details for GL-MAE.} Within the main manuscript, we have presented the linear and end-to-end segmentation settings for the \textit{BTCV dataset}, along with a description of the training process. Table~\ref{tab:configs} illustrates the various configurations utilized for each dataset. For the semi-supervised setting of the  \textit{BTCV dataset}, the model was trained for 3000 epochs, utilizing a batch size of 4 and a learning rate of 1e-4. For the \textit{MM-WHS dataset}, which is CT-based, the input volume was randomly cropped to [96, 96, 96], and the model was trained for 600 epochs with an initial learning rate of 1e-3 and a batch size of 2. The MRI-based \textit{BraTS dataset} had its input volume randomly cropped to [224, 224, 224], and the model was trained for 300 epochs with an initial learning rate of 1e-4. Due to the high resolution of the input volume, the batch size was set to 1. For the \textit{Covid-19-20 dataset}, the input volume was randomly cropped to [192, 192, 16], and the model was trained for 500 epochs, utilizing a batch size of 4 and a learning rate of 1e-4. Finally, for the \textit{MSD Task 07 dataset}, the input volume was cropped to [96, 96, 96], and the model was trained for 600 epochs with an initial learning rate of 1e-4, using a batch size of 2.

\subsection{COVID-19 lesion segmentation}
CT scans are a widely used tool for diagnosing COVID-19, but there is a scarcity of annotated data to train machine learning models for accurate segmentation of lesions. As shown in Table~\ref{tab:transferCovid19}, we evaluated the efficacy of a proposed method for segmenting lesions on the COVID-19 CT dataset. Our proposed method exhibits improved performance in lesion segmentation, increasing the score from 47.92\% to 49.88\% compared to the baseline and surpassing the competitive MAE3D. GL-MAE incorporates a feature learning approach that considers both global and local levels, leading to a significant improvement in model performance for lesion tasks. These findings suggest that our pre-trained model can capture valuable knowledge from unlabelled CT datasets to enhance disease diagnosis, demonstrating the promising potential of the proposed method in practical clinical settings.
\begin{table}[htb]
    \centering
   % \vspace{-5pt}
    \caption{Comparison on Covid-19 CT segmentation dataset with ViT-T as the backbone.}
    \label{tab:transferCovid19}
	\vspace{-5pt}
%	\scriptsize	
    \resizebox{0.75\linewidth}{!}{
    \begin{tabular}{cccc}
        \whline
        Method & Baseline & MAE3D & Ours \\
                \hline
        Dice Score(\%) &  47.92 & \underline{49.52} & \textbf{49.88}\\
        \whline
    \end{tabular}}
   \vspace{-5pt}
\end{table}

\subsection{Scaling up the pretraining dataset}
We assess whether GL-MAE can be scaled up to a larger pretraining dataset. Specifically, we employ the \textit{LUng Nodule Analysis 2016 (LUNA16)}\cite{murphy2009large,jacobs2014automatic,setio2015automatic,van2009automatic} dataset in our experiments, which can be obtained from the official website\footnote{\url{https://luna16.grand-challenge.org/Data/}}. Following the preprocessing steps outlined in~\cite{tang2022self}, we supplement the pretraining dataset with 886 additional CTs from LUNA16 to increase its scale. As presented in Table~\ref{tab:btcv_more_data}, we pretrained our proposed method on both the original pretraining dataset and the augmented dataset with LUNA16. Notably, our proposed method exhibited further improvements with the augmented dataset, even when trained for the same number of pretraining epochs.
\begin{table}[htb]
    \centering
    \caption{Dice score(\%) on the BTCV validation dataset by our proposed method under end-to-end segmentation evaluation. ViT-B is adopted and used as the backbone. Both models were trained for 400 epochs.}
	\vspace{-8pt}
    \label{tab:btcv_more_data}
    \resizebox{\linewidth}{!}{
    \begin{tabular}{ccccc}
        \whline
        \multicolumn{3}{c}{Pretraining dataset} & \multirow{2}{*}{Dataset scale} & \multirow{2}{*}{Dice score(\%)} \\
        BTCV & TCIA-Covid19 & LUNA16 &  & \\
        \hline
        \checkmark & \checkmark & - & $\sim 1,000$ & 79.70 \\
        \checkmark & \checkmark & \checkmark & $\sim 2,000$ & 81.41\greenp{1.71$\uparrow$}\\
        \whline
    \end{tabular}}
\end{table}

\subsection{Analysis of hyper-parameters.}
\noindent\textbf{Mask ratio.}
Table~\ref{tab:maskratio} presents the mask ratio of GL-MAE. We also investigated the optimal mask ratio for MAE models with ViT-B and ViT-T backbones, and the experimental results are shown in Figure~\ref{fig:maskratio_mae}. We observed that the best mask ratio for MAE3D is 0.6, which is consistent with the optimal mask ratio for GL-MAE.

\begin{table}[htb]
    \centering
    \caption{Dice score(\%) of BTCV dataset varying mask ratio.}
    \vspace{-8pt}
    \resizebox{0.64\linewidth}{!}{
    \begin{tabular}{c|ccc}
        \whline
         Mask ratio &  0.5 & 0.6 & 0.7\\
         \hline
         Dice score (\%) & 81.53 & \textbf{82.33} & 81.27\\ 
        \whline
    \end{tabular}
    }
    \label{tab:maskratio}
    \vspace{-5pt}
\end{table}
\begin{figure}[htb]
    \centering
    \includegraphics[width=0.75\linewidth]{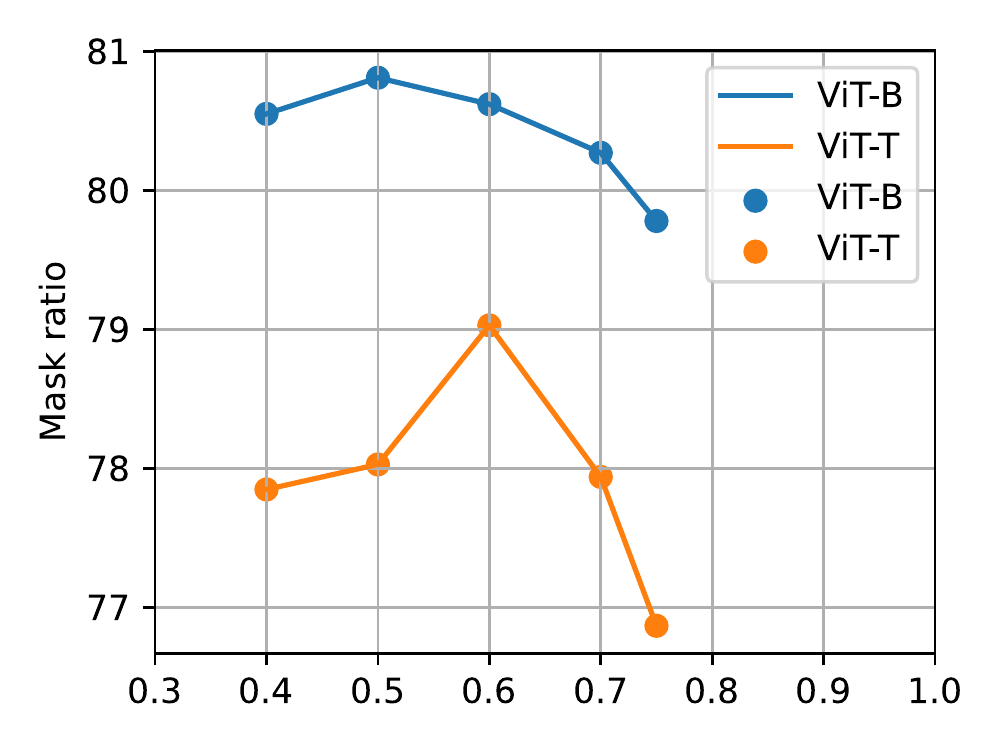}
    \caption{Dice score(\%) of MAE3D on the BTCV validation when mask ratio varies. All the model were pretrained with 500 epochs with a batch size of 128.}
    \label{fig:maskratio_mae}
\end{figure}

\noindent\textbf{Loss weight.} Based on the meanings of the losses, the four part losses \textbf{Eq.11} in the main paper can be grouped into two main categories, namely reconstruction loss $\mathcal{L}_R$,  and global-guided consistency loss $\mathcal{L}_C$. The values of these two loss types are on the same order of magnitude, as follows:
\begin{equation}\label{eq:rephrase_loss}
    \mathcal{L} = \mathcal{L}_R + \alpha\mathcal{L}_C,
\end{equation}
where $\alpha$ is the hyper-parameters to balance between the reconstruction and global-guided consistency loss. We conducted experiments to investigate the effect of increasing the weight of the consistency loss $\alpha$ from 0.1 to 1 and 10, and found that a weight of 1 provided the best results, as shown in Figure~\ref{fig:batchsize_lossweight}.

\noindent\textbf{Batch size.} We conducted an investigation into the impact of batch size on the performance of GL-MAE. Specifically, we tried batch sizes of 64, 128, and 256. As shown in Figure~\ref{fig:batchsize_lossweight}, increasing the batch size during pre-training had a positive impact on the downstream performance, which is consistent with the findings in~\cite{chen2020big}. This is because a larger batch size can provide a more accurate estimation of the overall data and accurate optimization direction.
\begin{figure}[htb]
    \centering
    \includegraphics[width=0.49\linewidth]{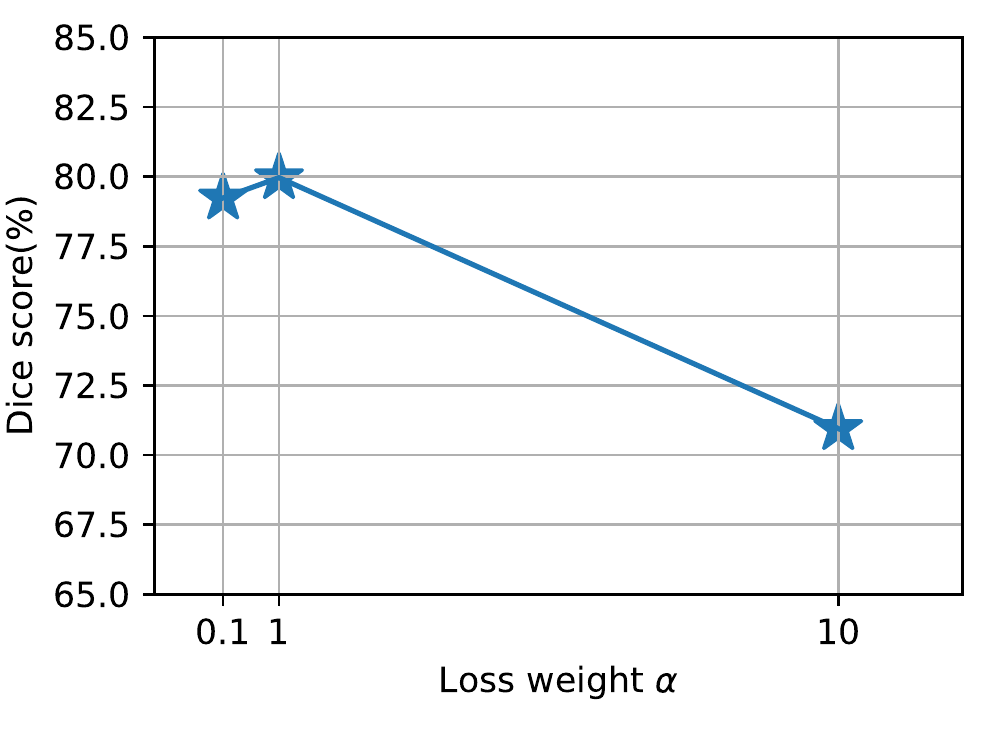}
    \includegraphics[width=0.49\linewidth]{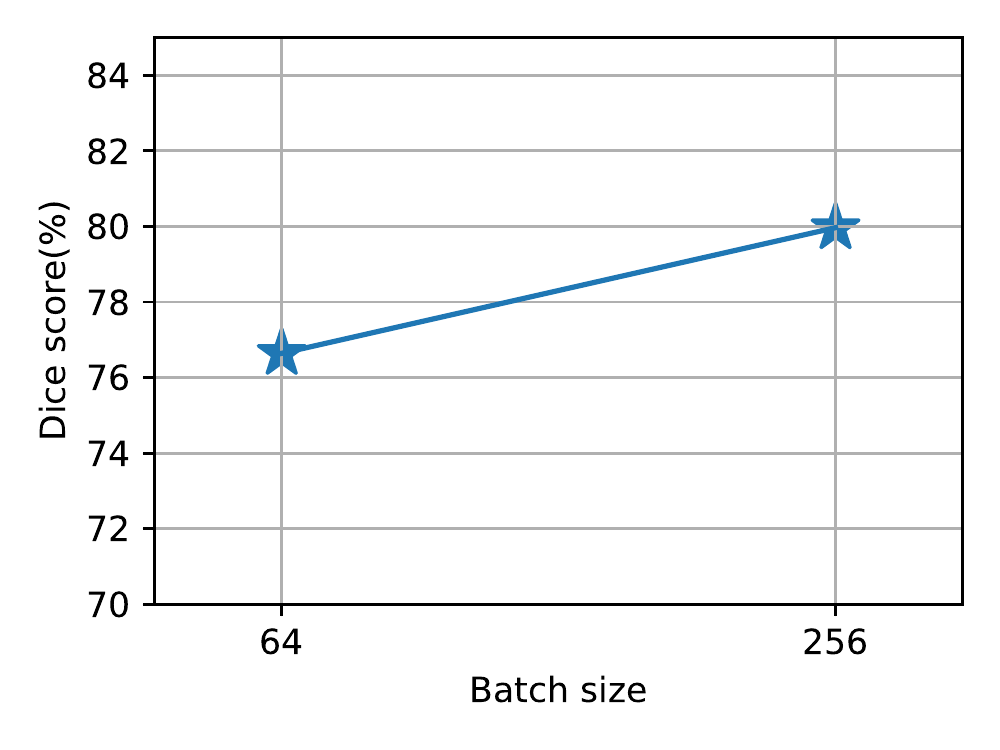}
    \caption{Left figure: Dice score of GL-MAE on the BTCV validation dataset when only varying the Loss weight $\alpha$ in Eq.~\ref{eq:rephrase_loss}. Right figure: Dice score of GL-MAE on the BTCV validation dataset when only increasing the batch size during pre-training. All model above were pre-trained with 100 epochs for saving time.}
    \label{fig:batchsize_lossweight}
\end{figure}

\subsection{Addition analysis of GL-MAE}

\noindent\textbf{Training process.} Figure~\ref{fig:training_process} illustrates the training process of the proposed method. More specifically, Figure~\ref{fig:training_process}(a) displays the final training loss curve, comprised of the reconstruction loss $L_R$, and the global-guided consistency loss function $L_C$. It is observed that the loss stability decreases as the number of epochs increases until 1000, and the dice score of the GL-MAE achieves 82.01\% on the BTCV validation dataset. When the model was further pretrained to 1600 epochs, the dice score could result in 82.33\%. Additionally, Figure~\ref{fig:training_process} indicates that the learning rate was adapted using a cosine scheduler.
\begin{figure}[htb]
    \centering
    \includegraphics[width=1.0\linewidth]{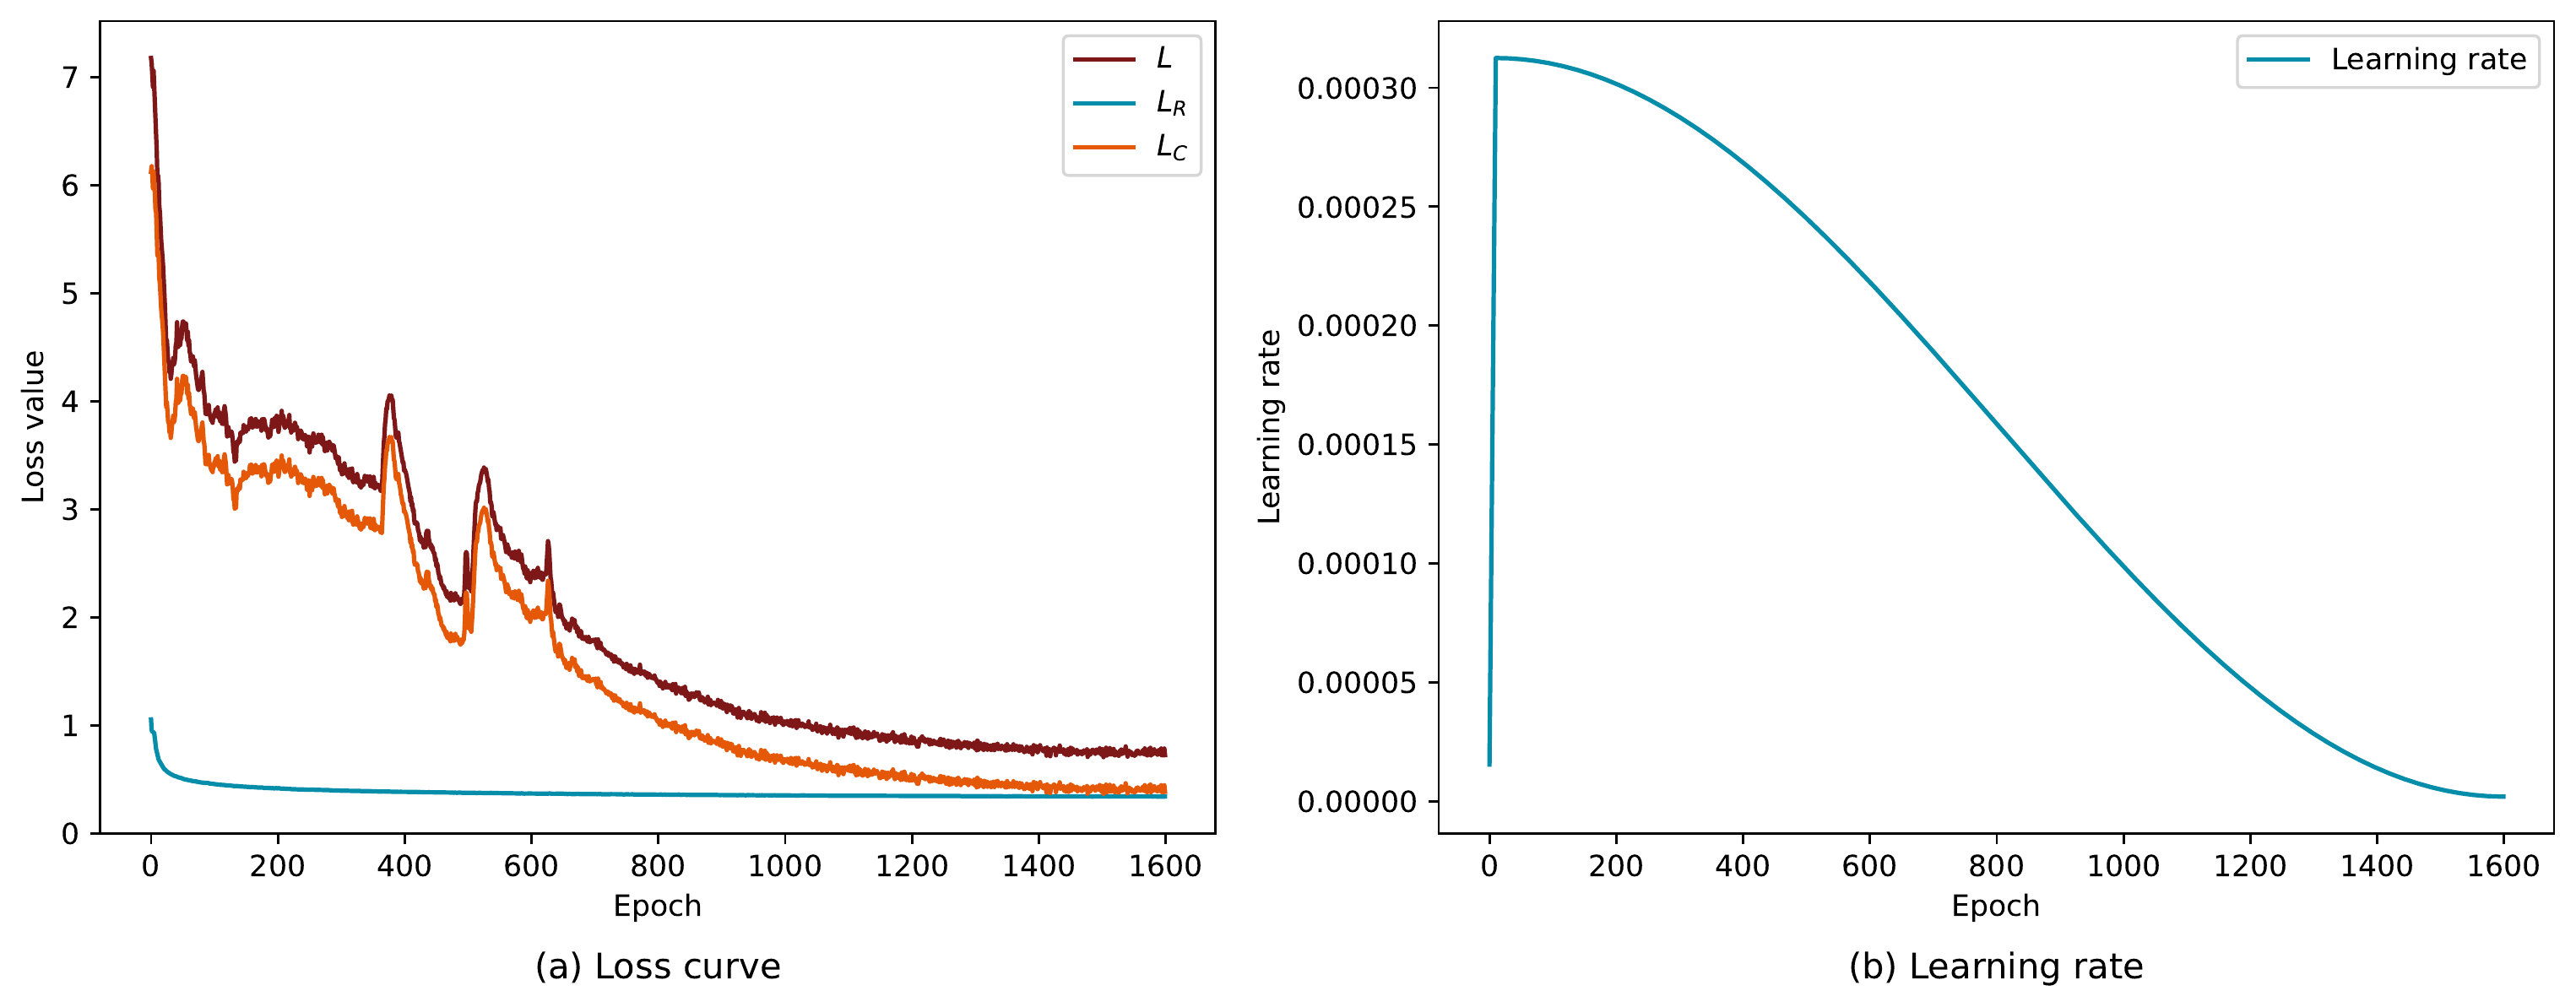}
    \vspace{-15pt}
    \caption{End-to-end segmentation performance on BTCV validation dataset when the pre-training epochs increase.}
    \label{fig:training_process}
\end{figure}

\begin{figure*}[htb]
    \centering
    \includegraphics[width=1.0\linewidth]{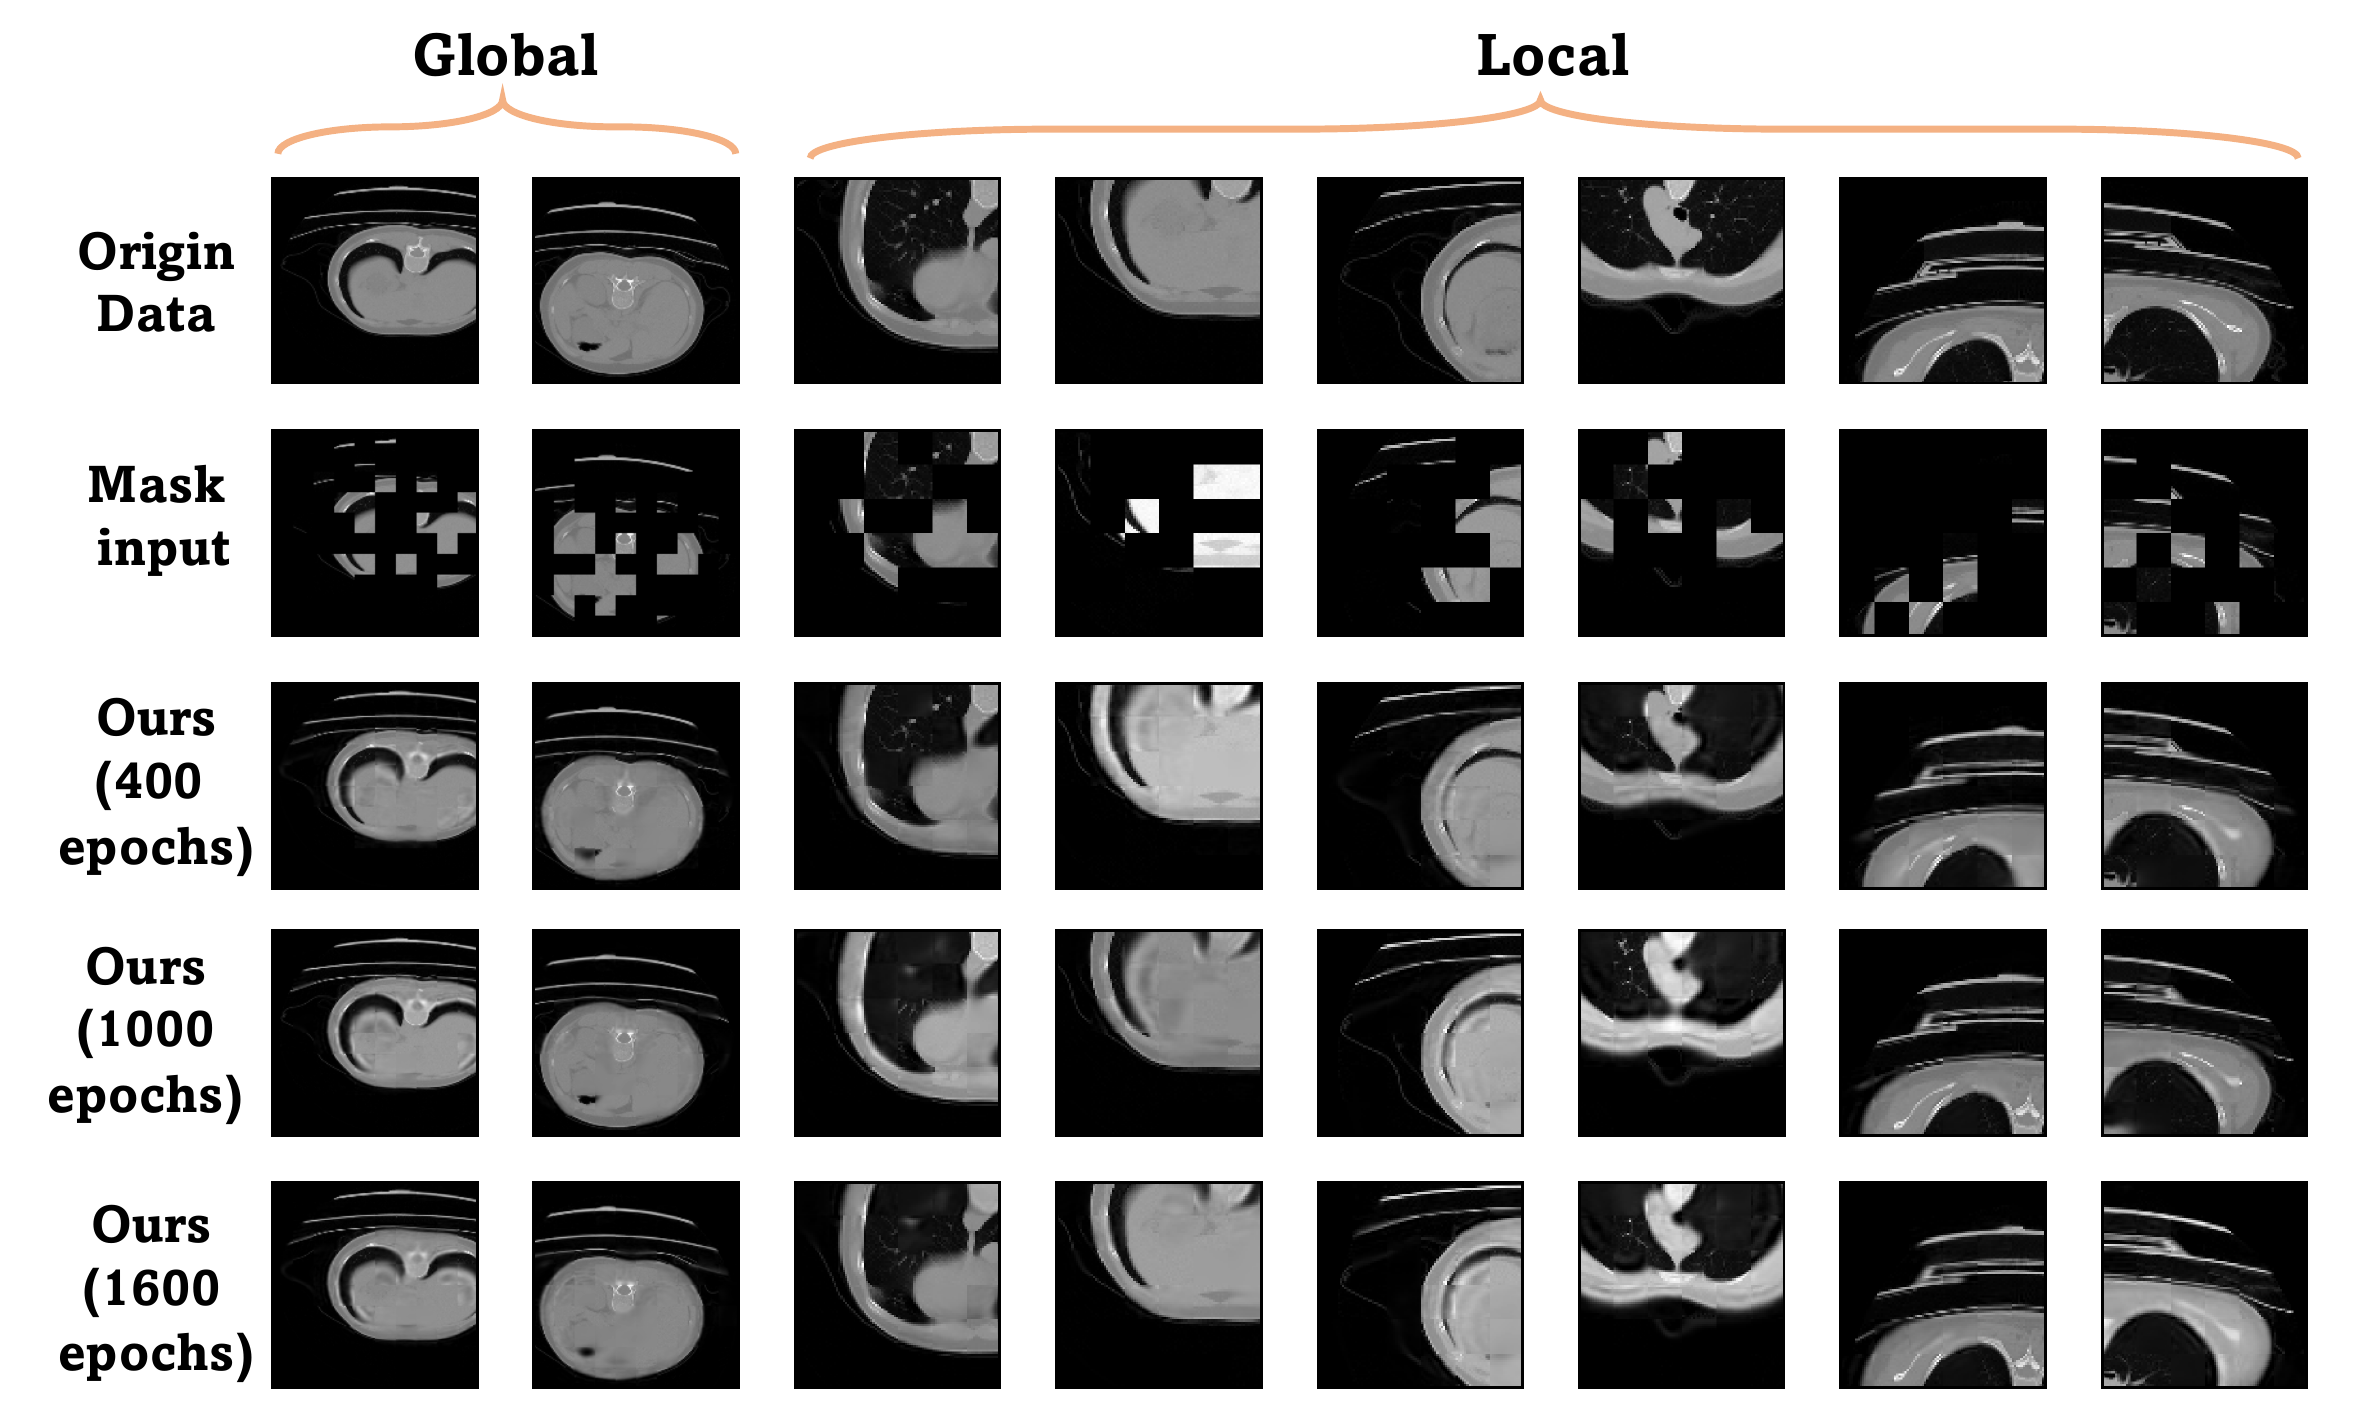}
    \vspace{-15pt}
    \caption{Reconstruction results of GL-MAE pretrained for 400, 1000, and 1600 epochs for the same input volume, respectively (Best viewed by zooming).}
    \label{fig:reconstruction}
\end{figure*}
\noindent\textbf{Reconstruction results.} This study presents examples of slices from CT scans that depict masks and their corresponding reconstruction results. These results were generated using our proposed method, which was pre-trained with 400, 1000, and 1600 epochs, as illustrated in Figures~\ref{fig:reconstruction}, respectively. These figures illustrate both global and local views for various input volumes, with each row consisting of two global views on the left column and six local views on the right column. All of the depicted slices pertain to distorted samples with a high mask ratio of 75\%. As illustrated in Figure~\ref{fig:reconstruction}, while the GL-MAE pertains to more epochs, the reconstruction for global and local views recovers the miss information better (Row 3$\sim$Row5). Our proposed method is capable of simultaneously reconstructing both local and global views, which is consistent with the MAE3D. As the model was trained for more epochs, the global and local reconstruction loss decreased and converged, leading to reconstruction results that were closer to the original data.

% \subsection{Visualization}
% 
% More visualization results could be found on Figure~\ref{fig:SegVisualizatoin_more}.
% \input{figures/segmentationResults_more.tex}
