# Supplementary material for: Advancing Volumetric Medical Image Segmentation via Global-Local Masked Autoencoder
Source: arXiv:2306.08913 source file (2023-08-23)
Supplement: Supplementary file 2 [file Supp_limitation_boarder.tex]

\section{Discussion}

\subsection{Impact of directly down-sampling the input volume as the input for MAE3D.}
We down-sampled the original sub-volumes to a sub-
volume of [96, 96, 96] and used it to pre-train the MAE. As shown in Figure~\ref{fig:mae_lowresolution}, the loss value of the down-sampling method decreased initially, similar to the cropped approach (used in our method and MAE3D baseline in our paper.), but was unable to continue decreasing the loss. This may be due to two factors. Firstly, the input volume was down-sampled too much from origin input volume (512 × 512 × 128 to 96 × 96 × 96), resulting in significant changes across different patches, making it difficult to recover based on neighboring patches. Secondly, too many details were lost, but the
changes inside the patches were still substantial. These factors made the mode hard to recover the missing pixel well. We also evaluated the performance of the down-sampling method on the BTCV validation dataset. We tried learning
rates of 3e-4, 1e-4, 5e-5, and 1e-5, and found that only a very low learning rate could prevent the model from experiencing gradient explosion and training failure. The results are pre-
sented in Table~\ref{tab:downsampleMAE}, which indicate that the down-sampling method performed significantly worse than the cropped approach used in our MAE3D baselines in the main paper and
our GL-MAE.
\begin{figure}[htb]
    \centering
    \includegraphics[width=0.75\linewidth]{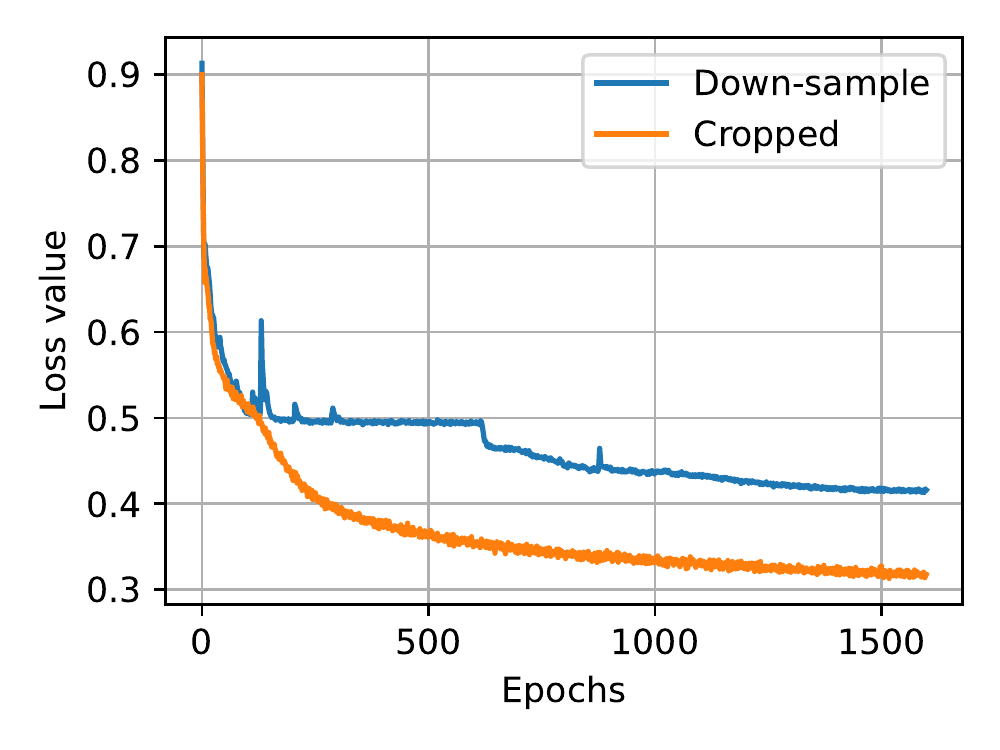}
    \caption{Loss value of the MAE3D on the BTCV validation dataset, backboned by ViT-B when using the down-sampling input volumes as the input.}
    \label{fig:mae_lowresolution}
\end{figure}
\begin{table}[htb]
    \centering
    \begin{tabular}{c|c}
        \whline
        Operation & Dice score(\%)\\
        \hline
         Cropped& \textbf{81.74}\\
         Downsample& 36.68 \\
        \whline
    \end{tabular}
    \caption{Dice score(\%) performance of the cropped and downsampling operation on the input volume. All model were evaluated under the same split and settings, including pre-trainng and fine-tuning epochs.}
    \label{tab:downsampleMAE}
\end{table}

\subsection{Broad impact}
Due to recent technological advancements in volumetric medical data sensing, there has been a surge of interest in machine learning algorithms that can perform analysis tasks on such data, as well as a growing number of applications for 3D imaging in fields such as Robotics and Medical Imaging~\cite{an2020ct}. This study focuses on the development of novel yet simple 3D deep learning pretraining algorithms for medical imaging in response to the pressing need for instant analysis systems that can aid the medical community in disease prevention, early detection, diagnosis, and treatment. Medical imaging plays a critical role in healthcare, and with the digitization of medical images, the hope that physicians can instantly analyze them with machine learning algorithms is becoming a reality. This is especially important in the current global pandemic, where radiography images provide a quick and rich diagnosis tool. However, the sheer expense of expert annotation required for supervised machine learning algorithms presents a challenge. To address this challenge, Self-Supervised approaches for representation learning from unlabelled data are necessary. The aim of this study is to provide the necessary tools for 3D image analysis and to aid physicians and radiologists in their diagnostic tasks from 3D scans while reducing the effort and cost of annotation required by these practitioners. Ultimately, this work is a small step towards leveraging machine learning for good in healthcare.

\subsection{Limitations and future work}
The foundation model is a widely recognized approach that exemplifies the potential of big data and large models\cite{touvron2023llama}. Self-Supervised Learning also benefits from the increasing volume of data and model capacity\cite{he2019moco}.
The limitation for GL-MAE is that the design of GL-MAE is relatively complex and may not be straightforward to scale to a larger datasets with higher capacity models, e.g., 100,000 CTs with ViT-Large. This is because the online encoder is fed by multiple masked local and global sub-volumes, and the model has four part losses, which need to tuned and results in expensive computation.

In future studies, we intend to extend our proposed method to larger datasets and higher-capacity models. While our research mainly focuses on pretraining method for downstream segmentation tasks, which are of significant interest to the medical community and have practical utility, we plan to conduct further investigations into other medical tasks, such as disease classification and lesion localization. Finally, we aim to broaden the scope of our framework to include cross-modality medical image analysis.
