# Supplementary material for: Advancing Volumetric Medical Image Segmentation via Global-Local Masked Autoencoder
Source: arXiv:2306.08913 source file (2023-08-23)
Supplement: Supplementary file 3 [file Supp_methods.tex]

\section{Method}\label{sec:supp_method}

We are providing additional information on the implementation of our proposed Global-local Masked Autoencoder. The first section provides a detailed explanation of our proposed algorithm, while the second section outlines and discusses the data augmentation process involved in our method.

\subsection{GL-MAE pre-training}
Algorithm~\ref{alg:overall} provides a step-by-step description of the key processes involved in our proposed method. Firstly, we initialized the momentum encoder with the student encoder and updated it in each iteration with a momentum ratio that is determined by a cosine scheduler. Next, let $\{\tau_1, \tau_2, \tau_m\} \subset\mathcal{T}$ represent the processing described in Algorithm~\ref{alg:dataAug}, and then we apply $\mathcal{T}$ to each input volume and generate both global and local views. These views were then fed into the encoder and momentum encoder for feature extraction. After obtaining their features, we utilized the proposed Global and Local Reconstruction loss functions and Global-guided Consistency Learning loss function to regulate the training process of the model. The momentum encoder would be updated based on the encoder with a momentum ratio $\mu$, which the initial value is 0.996 and increases to 1 during training with a cosine schedule.
\begin{algorithm}[!bth]
    \caption{The GL-MAE Algorithm}
    \label{alg:overall}
    \begin{algorithmic}[1]
        \REQUIRE An assembly CT dataset of $N$ data without labels.
        % \STATE \textbf{Input}: A assembly CT dataset without labels.
        \ENSURE Pre-trained encoder for downstream tasks.
        % \STATE \textbf{Output:} Pre-trained encoder for downstream tasks.
        \STATE // Sample a micro-batch \textit{X} from CT data each iteration.
        \FOR{$x \text{ in \textit{X}}$}
            % \STATE // Apply the augmentation Algorithm \textcolor{red}{1} in the supplementary materials over micro-batch of CT to obtain global and local views.
            % \STATE // Obtain local and global volumes.
            \STATE $\mathit{t_1, t_2}\sim \mathcal{T}$ // Sample transform 
            \STATE $V_l \gets \{v_l^{i}:v_l^{i}=t_1(x), i\in [1, q]$\}  
            \STATE $V_g \gets \{v_g^{i}:v_g^{i}=t_2(x), i\in [1, p]$\} 
            \STATE // Obtain local and global masked volumes.
            \STATE $\widetilde{V_l} \gets \{\widetilde{v_g^{i}}:v_l^{i}=t_m(v_l), v_l\in V_l$\} 
            \STATE $\widetilde{V_g} \gets \{\widetilde{v_l^{i}}:v_g^{i}=t_m(v_g), v_g\in V_g$\} 
            % \STATE $\widetilde{V}\gets \widetilde{V_l} \cup \widetilde{V_g}$
            \FOR{$v_g \text{ in } \textit{V}_g$}
                \FOR{$\widetilde{v_l}, \widetilde{v_g}, v_l, v_g \text{ in } \widetilde{V_l} \cup \widetilde{V_g}\cup V_l \cup V_g$}
                    \STATE Obtain embeddings $\widetilde{Z_l}$ and $\widetilde{Z_g}$ by \textbf{Eq.1}
                    \STATE Obtain embeddings $y_l$ and $y_g$ by \textbf{Eq.2}
                    \STATE // Reconstruction by \textbf{Eq}.3 and \textbf{Eq.4}.
                    \STATE $\mathcal{L}_\mathcal{R}^l(y_l, v_l)$, $\mathcal{L}_\mathcal{R}^g(y_g, v_g)$ 
                    \STATE Obtain embeddings $E_f$, $E_g$ and $E_l$ by \textbf{Eq.6}.
                    \STATE // Global-to-global consistency by \textbf{Eq.9}.
                    \STATE $\mathcal{L}_\mathcal{C}^{gg}({E}_f, \widetilde{{E}_l})$
                    \STATE // Global-to-local consistency by \textbf{Eq.10}.
                    \STATE $\mathcal{L}_\mathcal{C}^{gl}({E}_f, \widetilde{{E}_g})$ 
                    % \STATE  // 
                    \STATE Calculate the overall loss $\mathcal{L}$.
                    \STATE Update parameters of s($\cdot$) and momentum encoder m($\cdot$) with \textbf{Eq.5}
                    % = $\mathcal{D}(s(\widetilde{v_g};\theta_s))$
                \ENDFOR
            \ENDFOR
            % \STATE Apply  to obtain reconstructed views $\{y_g, y_l\}$ 
            % \STATE // \textcolor{mygreen}{To obtain global and local reconstructed views.}
            % \STATE $y_g, y_l$ // Eq.\textcolor{red}{\ref{eq:y}}
        \ENDFOR
    \end{algorithmic}
\end{algorithm}

\noindent\textbf{Why don't directly use Global views as the input for MAE3D?}
The reason for not using Global views directly as the input for MAE3D is that volumetric data, such as CT scans, are typically large in size and need to be broken down into several patches for further processing. Additionally, the reconstruction task for MAE3D is to predict the missing value in a pixel, and downsampling the input volume can result in low resolution and the loss of important details, particularly in small organs and tumors. Therefore, previous work has used cropped volumes from the input volumes to maintain resolution and details. We conducted experiments to analyze the impact of downsampling the input volumes and using them as input. Please refer to Table~\ref{tab:downsampleMAE} in Section Discussion for more information.

\subsection{Data augmentation in the pre-training stage}
Algorithm \ref{alg:dataAug} described the detailed implementation of the data augmentation process. We designed two distinct procedures $\tau_1$ and $\tau_2$ for data augmentation that cater to local and global views. To obtain a global view, we apply $\tau_2$ by first establishing a $\rm{global\_scale\_factor}$  within the range of [0.5, 1] and cropping a sub-volume by a random $\rm{global\_scale\_factor}$. Additionally, we set $\rm{global\_size}$ to [160, 160, 160] and \textit{downsample} the input volume to this size. For the local view, we apply $\tau_1$ by setting a $\rm{local\_scale\_factor}$ within the range of  [0.25, 0.5] and then crop a sub-volume by a random $\rm{local\_scale\_factor}$. Finally, we set $\rm{local\_size}$ to [96, 96, 96] and resize the local cropped sub-volume to this size. For each input volume $x$, we apply the data processing operation $p$ times and $q$ times to obtain $p$ global views and $q$ local views, respectively. To obtain the masked sub-volumes $\widetilde{V}$, following ~\cite{chen2023masked}, we apply $\tau_m$ by randomly masking the patches from the local and global sub-volumes. 

\vspace{-5pt}
\begin{algorithm}[H]
    \footnotesize
    \caption{Pseudocode of data augmentation in PyTorch-like style.}
    \label{alg:dataAug}
    \begin{algorithmic}[0]
        \STATE \textcolor{mygreen}{\# \textbf{Input}: volume, global\_scale\_factor, local\_scale\_factor, local\_crop\_numbers, global\_size, local\_size}
        \STATE \textcolor{mygreen}{\$ \textbf{Output}: crops}
		\STATE \textcolor{mygreen}{\# volumn: loading a sample from the 3D CT datasat used for pretraining, which has been processed by spacing, scaleIntensity etc. }
		\STATE \textcolor{mygreen}{\# global\_scale\_factor, local\_scale\_factor: factors to scale the image.}
		\STATE \textcolor{mygreen}{\# global\_crop\_numbers: numbers of cropped volume, e.g., 2. }
		\STATE \textcolor{mygreen}{\# local\_crop\_numbers: numbers of cropped volume, e.g., 8. }
		\STATE \textcolor{mygreen}{\# global\_size, local\_size: size for global and local sub Volume.}
		\STATE
		\STATE \textcolor{mygreen}{\# Define transforms $\tau_1$ for generating local sub-volumes}
		\STATE local\_transform = Compose([
		\STATE \quad\quad RandScaleCropd(local\_scale\_factor), \STATE \quad\quad Resized(local\_size)])	
        \STATE \textcolor{mygreen}{\# Define transforms $\tau_2$ for generating local sub-volumes}
		\STATE global\_transform = Compose([
		\STATE \quad\quad RandScaleCropd(global\_scale\_factor), \STATE \quad\quad Resized(global\_size)])		
		\STATE crops = [] \textcolor{mygreen}{\# Process of generating the expected sub volumes}
		\STATE for iter in range(global\_crop\_numbers):
		\STATE \quad crops.append(global\_transforms(volume))
		\STATE for iter in range(local\_crop\_numbers):
		\STATE \quad crops.append(local\_transform(volume))
    \end{algorithmic}
\end{algorithm}
% \vspace{-10pt}

\noindent\textbf{How much overlap between the local and global views?}
To ensure consistency learning between the local and global views, it is important that they share an overlap region. To determine the overlap region ratio between the local and global views generated from the same data during one epoch of training, we conducted an analysis, and the results are presented in Table~\ref{tab:gl_ratio}. We carefully selected hyper-parameters, including randomly selecting a scale ratio to scale the input data, to ensure that the overlap ratio between the local and global views is reasonable. The average overlap ratio (\%) for the local view $\rm{Overlap}$ was computed over all $q$ local crop $v_l$ global crop $v_g$ for the unlabelled dataset $\mathcal{D}$ with $N$ input data during one epoch using the following equation:

\begin{equation}\label{localview_ratio}
    \rm{Overlap}(\mathcal{D}):=\frac{1}{N|V_g||V_l|} \sum_{i=1}^{N} \sum_{v_g^i\in V_g} \sum_{v_l^i\in V_l}\frac{v_l^{i} \cap v_g^{i}}{v_l^{i}} \times 100.
\end{equation}
Table~\ref{tab:gl_ratio} demonstrates that the global view remains stable at $377\times296\times53$, while the shape of the local view varies from $126\times99\times18$ to $252\times197\times36$ as the $\rm{local\_scale\_factor}$ is modified. Additionally, as the $\rm{local\_scale\_factor}$ is increased from 0.25 to 0.5, the overlap ratio for local $\rm{overlap}$ increases from 62.57\% to 70.00\%. It can be concluded that the local and global views will share the overlap region most of the time, thereby ensuring semantic consistency. To enhance the model's ability to learn robust representation, we adopted a strategy of randomly selecting $\rm{local\_scale\_factor}$ each iteration from the range of [0.25, 0.5]. 

For a more intuitive observation of the overlap situation between the local and global views from the same data, we define a measurement method called $\textrm{Hit}$ in the equation:
\begin{equation}\label{eq:hit}
    \rm{Hit}(\mathcal{D}):= \frac{1}{N} \sum_{i=1}^{N} \sum_{v_g^i\in V_g} \sum_{v_l^i\in V_l} \frac{sgn(v_l^{(i)} \cap v_g^{(i)})}{|V_l||V_g|} \times 100
\end{equation}
\jiaxin{where the $sgn$ represents the Sign function. The 
$\rm{Hit}$ metric can be utilized to measure the frequency of overlap across the entire dataset. It can be observed from the 4th row in Table~\ref{tab:gl_ratio} that the overlap between the global and local views from the same volume is most frequent when we increase the  $\rm{local\_scale\_factor}$}.
\begin{table}[h]
    \centering
    \caption{Average patch size, Overlap(\%), and Hit(\%) of the local and global view from the same input data for one epoch when varies the $\rm{local\_scale\_factor}$.}\label{tab:gl_ratio}
    % \small
    \resizebox{1\linewidth}{!}{
    \begin{tabular}{ccccc}
         \whline
         Metric & 0.25 & 0.5 & 0.25$\sim $0.5 \\ 
         \hline
        Global size & $381\times297\times54$ & 
        $377\times296\times53$ &
        $377\times296\times53$\\
        Local size& $126\times99\times18$ & 
        $252\times197\times36$ & $189\times148\times27$\\
         \hline
         % \multirow{1}{*}{Overlap}& Global & $2.46\pm1.65$ & $4.45\pm2.57$ & $11.15\pm5.15$ & $21.63\pm8.11$ & $8.82\pm5.56$\\
         Overlap(\%) & $62.57\pm36.69$ & $70.00\pm24.13$& $66.89\pm30.00$\\
         % \hline
         \cdashline{1-5}
         Hit(\%) & 89.51 & 100 & 97.12\\
         % & Local view & 100 & & & & \\
         \whline\\
    \end{tabular}
    }
\end{table}

% Factor 0.25, 0.5, 0.25~0.5
% x,y,z
% remove overlap global

% \begin{table}[h!]
%     \centering
%     \caption{Average View size, Overlap(\%), and Hit(\%) of the local and global view from the same input data for one epoch when varies the $\rm{local\_scale\_factor}$.}\label{tab:gl_ratio}
%     \small
%     \resizebox{14cm}{!}{
%     \begin{tabular}{ccccccc}
%          \whline
%          Metric & Factor & 0.25 & 0.3 & 0.4 & 0.5 & 0.25$\sim $0.5 \\ 
%          \hline
%         \multirow{2}{*}{Size} & Global & $176.60\pm32.10$ & $177.02\pm30.92$ & $177.38\pm31.86$& $177.38\pm31.86$ & $177.38\pm31.86$\\
%          & Local & $60.10\pm7.92$ & $72.13\pm9.51$ & $95.90\pm12.72$& $119.45\pm15.90$ & $88.57\pm15.74$\\
%          \hline
%          \multirow{2}{*}{Overlap}& Global & $2.46\pm1.65$ & $4.45\pm2.57$ & $11.15\pm5.15$ & $21.63\pm8.11$ & $8.82\pm5.56$\\
%          Overlap & Local & $62.57\pm36.69$ & $65.95\pm33.62$ & $69.76\pm28.20$ & $70.00\pm24.13$& $66.89\pm30.00$\\
%          % \hline
%          \cdashline{1-7}
%          Hit & - & 89.51 & 94.27 & 99.3 & 100 & 97.12\\
%          \whline\\
%     \end{tabular}}
% \end{table}
