# Supplementary material for: Advancing Volumetric Medical Image Segmentation via Global-Local Masked Autoencoder
Source: arXiv:2306.08913 source file (2023-08-23)
Supplement: Supplementary file 5 [file supp_gl_ratio.tex]

\begin{table}[h]
    \centering
    \caption{Average patch size, Overlap(\%), and Hit(\%) of the local and global view from the same input data for one epoch when varies the $\rm{local\_scale\_factor}$.}\label{tab:gl_ratio}
    % \small
    \resizebox{1\linewidth}{!}{
    \begin{tabular}{ccccc}
         \whline
         Metric & 0.25 & 0.5 & 0.25$\sim $0.5 \\ 
         \hline
        Global size & $381\times297\times54$ & 
        $377\times296\times53$ &
        $377\times296\times53$\\
        Local size& $126\times99\times18$ & 
        $252\times197\times36$ & $189\times148\times27$\\
         \hline
         % \multirow{1}{*}{Overlap}& Global & $2.46\pm1.65$ & $4.45\pm2.57$ & $11.15\pm5.15$ & $21.63\pm8.11$ & $8.82\pm5.56$\\
         Overlap(\%) & $62.57\pm36.69$ & $70.00\pm24.13$& $66.89\pm30.00$\\
         % \hline
         \cdashline{1-5}
         Hit(\%) & 89.51 & 100 & 97.12\\
         % & Local view & 100 & & & & \\
         \whline\\
    \end{tabular}
    }
\end{table}

% Factor 0.25, 0.5, 0.25~0.5
% x,y,z
% remove overlap global

% \begin{table}[h!]
%     \centering
%     \caption{Average View size, Overlap(\%), and Hit(\%) of the local and global view from the same input data for one epoch when varies the $\rm{local\_scale\_factor}$.}\label{tab:gl_ratio}
%     \small
%     \resizebox{14cm}{!}{
%     \begin{tabular}{ccccccc}
%          \whline
%          Metric & Factor & 0.25 & 0.3 & 0.4 & 0.5 & 0.25$\sim $0.5 \\ 
%          \hline
%         \multirow{2}{*}{Size} & Global & $176.60\pm32.10$ & $177.02\pm30.92$ & $177.38\pm31.86$& $177.38\pm31.86$ & $177.38\pm31.86$\\
%          & Local & $60.10\pm7.92$ & $72.13\pm9.51$ & $95.90\pm12.72$& $119.45\pm15.90$ & $88.57\pm15.74$\\
%          \hline
%          \multirow{2}{*}{Overlap}& Global & $2.46\pm1.65$ & $4.45\pm2.57$ & $11.15\pm5.15$ & $21.63\pm8.11$ & $8.82\pm5.56$\\
%          Overlap & Local & $62.57\pm36.69$ & $65.95\pm33.62$ & $69.76\pm28.20$ & $70.00\pm24.13$& $66.89\pm30.00$\\
%          % \hline
%          \cdashline{1-7}
%          Hit & - & 89.51 & 94.27 & 99.3 & 100 & 97.12\\
%          \whline\\
%     \end{tabular}}
% \end{table}
